# Supplementary material for: TeaMs-RL: Teaching LLMs to Generate Better Instruction Datasets via Reinforcement Learning
Source: arXiv:2403.08694 source file (2025-03-01)
Supplement: Supplementary file 1 [file experiments-additional.tex]

\subsection{Comparison Experiments on LM Eval Benchmakrs}

To comprehensively examine the effectiveness of our method, we carry out experiments on LM-Eval benchmark\footnote{\url{https://huggingface.co/spaces/HuggingFaceH4/open_llm_leaderboard}}$^{,}$\footnote{\url{https://github.com/EleutherAI/lm-evaluation-harness}}, the LM-Eval benchmark stands as a prominent tool for assessing LLM performance. It encompasses a suite of sub-benchmarks: (1) AI2 Reasoning Challenge (ARC) benchmark~\citep{clark2018think}: The benchmark introduces a fresh question set, text corpus, and baselines, all strategically curated to foster and propel AI research in the realm of advanced question answering, setting a significantly higher bar for knowledge and reasoning capabilities compared to previous challenges. (2) HellaSwag benchmark~\citep{zellers2019hellaswag}: The benchmark introduces a challenging dataset, revealing that even state-of-the-art models struggle with commonsense inference, as evidenced by the significant performance gap between humans ($95\%$ accuracy) and models ($48\%$), achieved through adversarial filtering, a robust data collection paradigm that selects adversarial machine-generated wrong answers by scaling up the length and complexity of dataset examples to a 'Goldilocks' zone where the text generated is absurd to humans yet often misclassified by models. (3) Massive Multitask Language Understanding (MMLU) benchmark~\citep{hendrycks2020measuring}: The benchmark serves as a comprehensive assessment of a text model's multitask accuracy, encompassing a total of 57 distinct tasks. These tasks span various domains, including elementary mathematics, US history, computer science, law, and others. Achieving a high level of accuracy on this benchmark necessitates a strong grasp of world knowledge and strong problem-solving capabilities. (4) Truth Question-Answering (TruthQA) benchmark~\citep{lin2022truthfulqa}: The benchmark encompasses a diverse array of 817 questions distributed across 38 distinct categories, encompassing a wide spectrum of domains such as health, law, finance, and politics. 

In our comparison experiments, we take the same setting as the LM-Eval benchmarks shown, e.g., 25 shots for ARC, 10 shots for HellaSwag, 5 shots for MMLU, and 0 shot for TruchfulQA.

\begin{comment}
\begin{itemize}
\item[$\bullet$] \textbf{ARC}: AI2 Reasoning Challenge (25-shot) - a set of grade-school science questions.
\item[$\bullet$] \textbf{HellaSwag}: HellaSwag (10-shot) - a test of commonsense inference, which is easy for humans (~95\%) but challenging for SOTA models.
\item[$\bullet$] \textbf{MMLU}: MMLU (5-shot) - a test to measure a text model's multitask accuracy. The test covers 57 tasks including elementary mathematics, US history, computer science, law, and more.
\item[$\bullet$] \textbf{TruthfulQA}: TruthfulQA (0-shot) - a test to measure a model’s propensity to reproduce falsehoods commonly found online. Note: TruthfulQA in the Harness is actually a minima a 6-shots task, as it is prepended by 6 examples systematically, even when launched using 0 for the number of few-shot examples.
\end{itemize}    
\end{comment}

% We compared our method with WizardLM-7b\footnote{\url{https://huggingface.co/TheBloke/WizardLM-7B-HF}} and Llama-2-chat-7b\footnote{\url{https://huggingface.co/meta-llama/Llama-2-7b-chat-hf}} models on this benchmark. As shown in Figure~\ref{fig:compared-with-llama-2-chat-7b}, we trained a llama-2-chat-7b model as our model (named TeaMs-RL-7b-v2.0) with our dataset, the experimental results demonstrate that our model performs better than the llama-2-chat-7b model on overall performance, especially on MMLU and TruthQA tasks, our method shows significantly better than the llama-2-chat-7b model.

 \subsection{Compare with WizardLM-7b Model}
\label{sec:lama1}
 % We also trained a llama-1-7b model as our model (named TeaMs-RL-7b-v1.0) with our dataset. As shown in Figure~\ref{fig:compared-with-WizardLM-llama-1-7b}, our method perform better than llama-1-7b models on various tasks, and also our method present similar performance results with WizardLM-7b models. However, as shown in Figure~\ref{fig:compared-with-WizardLM-number-instructions} (a), the size of the dataset that we used to train our model is about one-sixteenth of that WizardLM used, and as shown in Figure \ref{fig:compared-with-WizardLM-number-instructions} (b), WizardLM asks about GPT models forty times as many times as we do, which could be very expensive to collect that such dataset.

Furthermore, we extended our comparative analysis to a llama-1-7b model denoted ``TeaMs-RL-7b-v1.1," trained on our dataset of 17,878 instruction-response pairs. As shown in Figure~\ref{fig:compared-with-WizardLM-llama-1-7b-gpt-ans}, our method shows superior average performance over llama-1-7b models and on par with WizardLM-7b models~\footnote{\url{https://huggingface.co/TheBloke/WizardLM-7B-HF}}$^{,}$\footnote{In our experimental setup, all models are configured with a float16 format. {We compare to WizardLM-7b since both this approach and ours use llama-1-7b as the base model. Notably, WizardLM-7B queried ChatGPT 624,000 times for responses, whereas our method queried open-source WizardLM13B 371 times during policy training and ChatGPT 35,756 times. As WizardLM13B has similar capabilities to ChatGPT, our total queries are substantially fewer. Therefore, we believe the comparison is fair in terms of matched base model and vastly lower query amount.}}. We also fine-tuned a ``TeaMs-RL-7b-v1.0'' model on our previous 15,392-sample dataset, attaining performance comparable to WizardLM-7b.
\hl{The slightly lower HellaSwag/ARC results seem to originate from the initial Alpaca instruction set prioritizing multi-tasking over specialization, evidenced by similar WizardLM outcomes (Figs. ~\ref{fig:compared-with-llama-2-chat-7b} and \ref{fig:compared-with-WizardLM-llama-1-7b-gpt-ans}).} See Appendix \ref{appenidx:comparison-experiments-TeaMs-RL-7b-v10} for details.

It is crucial to underscore a salient aspect of our methodology in relation to data utilization. The dataset employed for training our model is approximately one-fourteenth the size of the dataset utilized by WizardLM, as illustrated in Figure \ref{fig:compared-with-WizardLM-number-instructions-gpt-ans} (a). Furthermore, Figure~\ref{fig:compared-with-WizardLM-number-instructions-gpt-ans} (b) highlights the discernible difference in the query count posed to GPT models between our method and WizardLM, with the latter soliciting GPT models for responses at a rate seventeen times higher. This marked contrast underscores the cost-effectiveness of our data collection approach, which mitigates the expenses associated with dataset acquisition. It highlights that our method is a more economically viable and sustainable strategy for training LLMs.

\begin{figure}[tb!]
 \centering
 % \vspace{-30pt}
 % \subcaptionbox{}
 {
\includegraphics[width=0.99\linewidth]{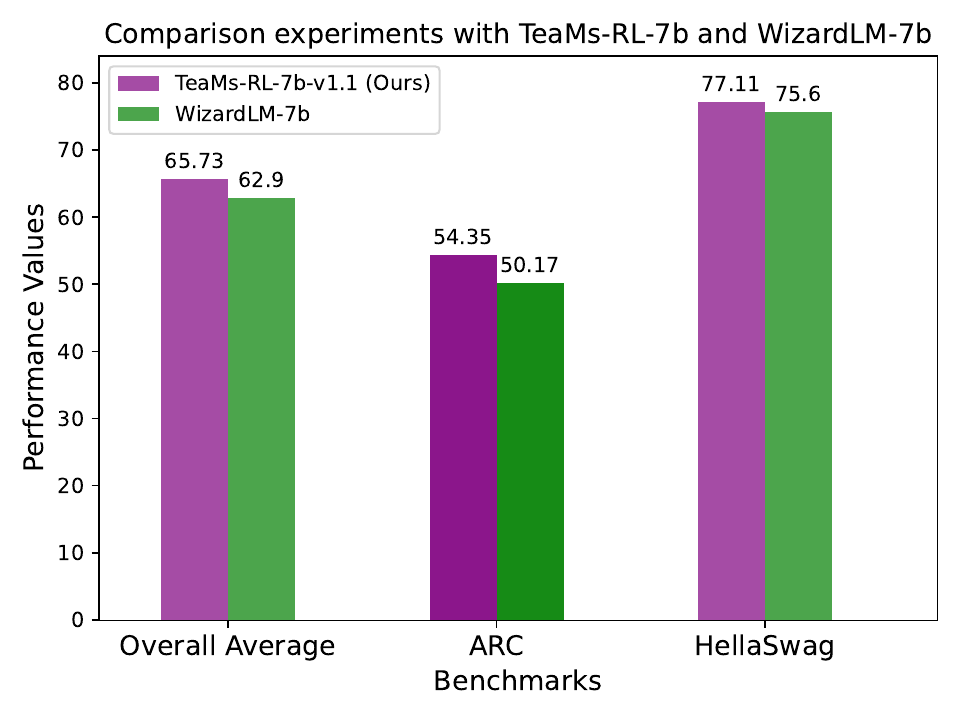}
}
    % \vspace{-10pt}
 	\caption{\normalsize Compare our method with WizardLM 7B on LM-Eval Benchmarks. 
 	} 
  \label{fig:compared-with-teamsRL-WizardLM-7b-gpt-ans}
 \end{figure}

  \begin{figure}[tb!]
 \centering
 % \vspace{-15pt}
 \subcaptionbox{}
 {
\includegraphics[width=0.99\linewidth]{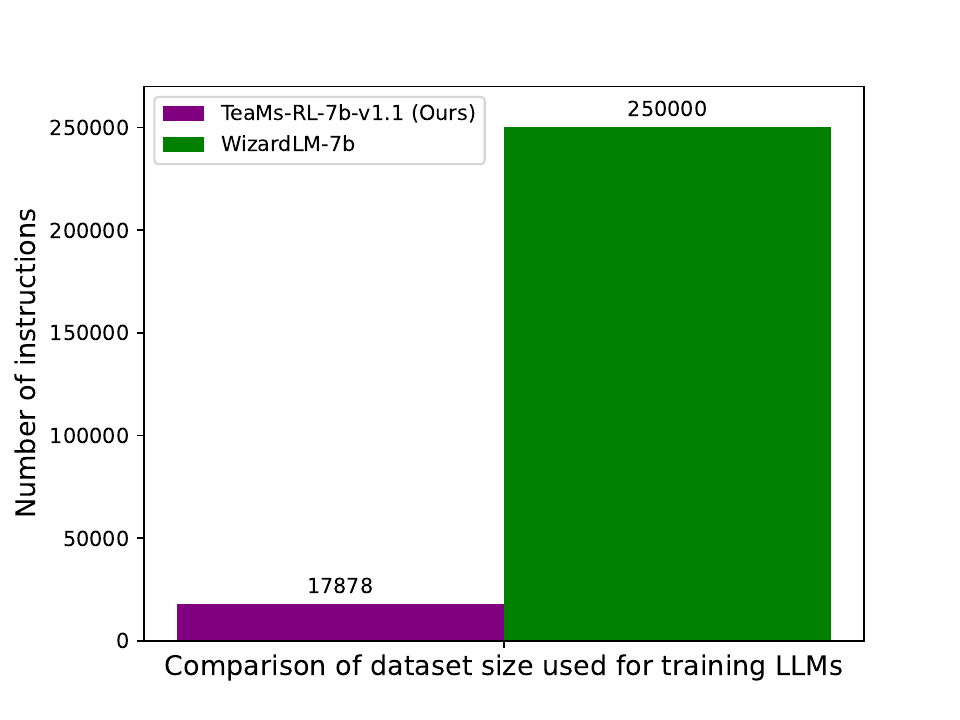}
}
 \subcaptionbox{}
 {
\includegraphics[width=0.99\linewidth]{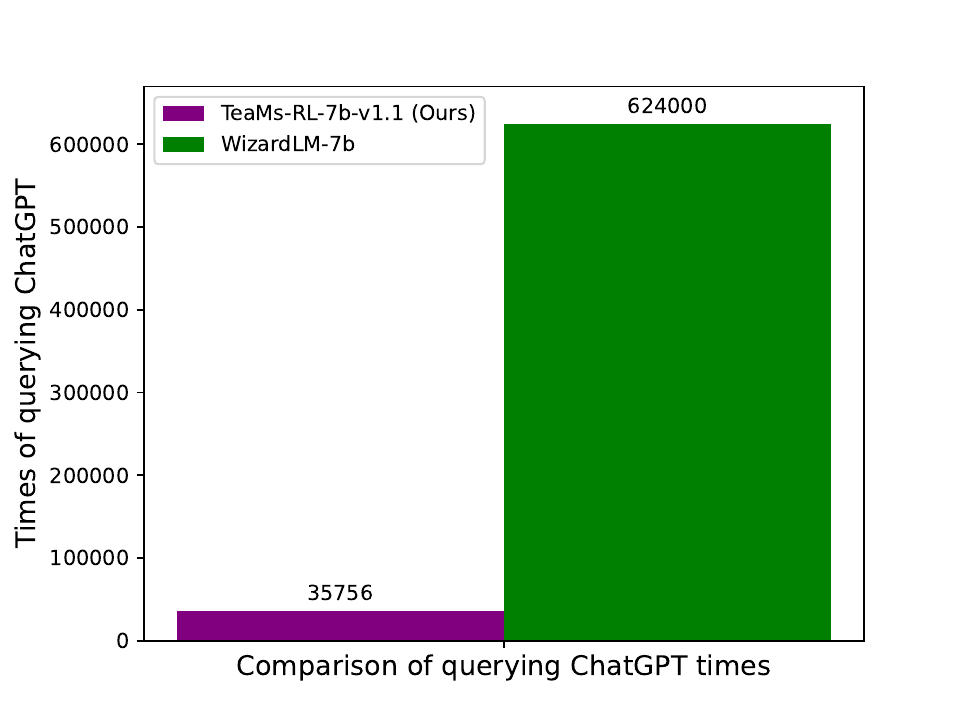}
}
    % \vspace{-5pt}
 	\caption{\normalsize Compare with WizardLM 7B on dataset size used for training LLMs and querying times of advanced LLMs. 
 	} 
  \label{fig:compared-with-teams-RL-WizardLM-number-instructions-gpt-ans}
    % \vspace{-10pt}
 \end{figure} 
% \vspace{-5pt}

\begin{figure}[tb!]
 \centering
 % \vspace{-30pt}
 % \subcaptionbox{}
 {
\includegraphics[width=0.99\linewidth]{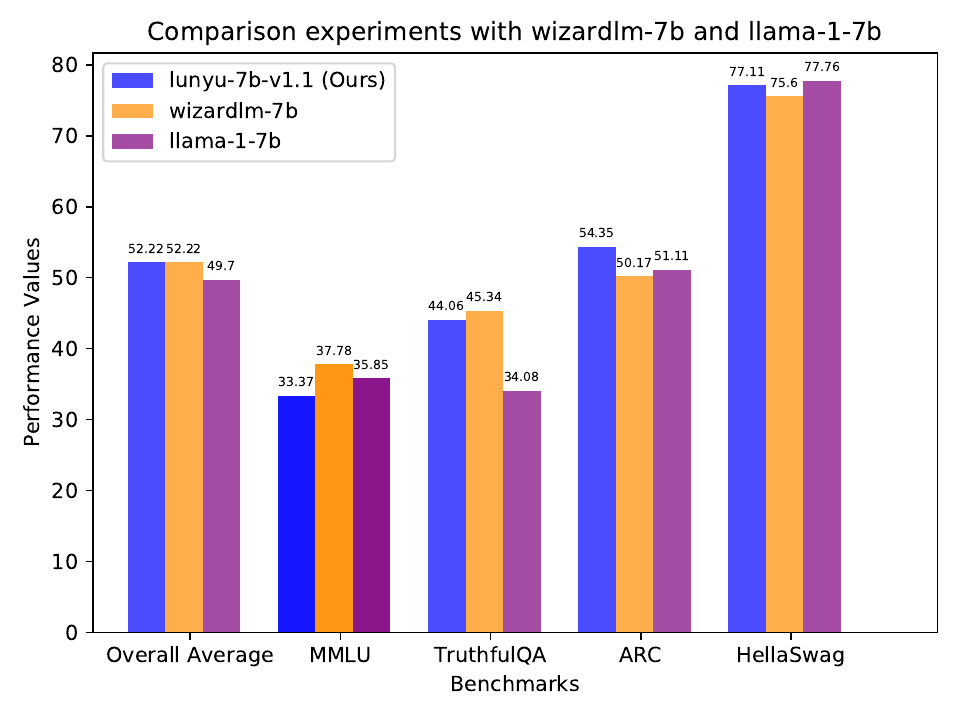}
}
    \vspace{-10pt}
 	\caption{\normalsize Compare our method with WizardLM 7B and llama-1-7b on LM-Eval Benchmarks. 
 	} 
  \label{fig:compared-with-WizardLM-llama-1-7b-gpt-ans}
 \end{figure}

\begin{comment}
 \begin{figure}[htbp!]
 \centering
 % \subcaptionbox{}
 {
\includegraphics[width=0.97\linewidth]{files/figures/compare-WizardLM/compare_TeaMs-RL_WizardLM.pdf}
}
    \vspace{-0pt}
 	\caption{\normalsize Compare our method with WizardLM 7B on LM Eval Benchmarks. 
 	} 
  \label{fig:compared-with-WizardLM}
 \end{figure} 
\end{comment}

  \begin{figure}[tb!]
 \centering
 \vspace{-15pt}
 \subcaptionbox{}
 {
\includegraphics[width=0.99\linewidth]{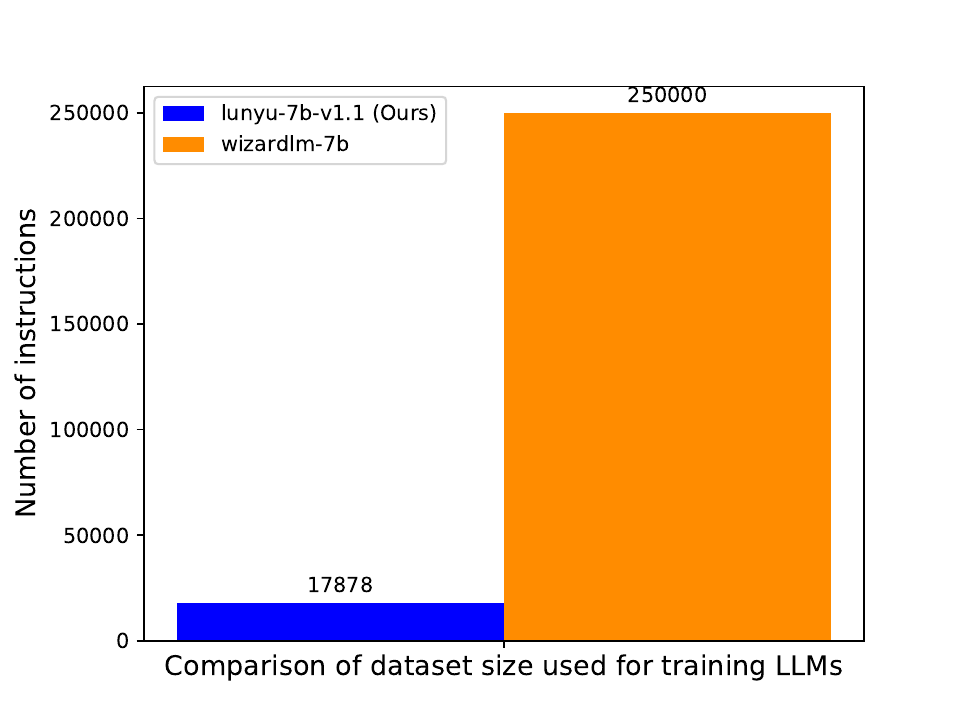}
}
 \subcaptionbox{}
 {
\includegraphics[width=0.99\linewidth]{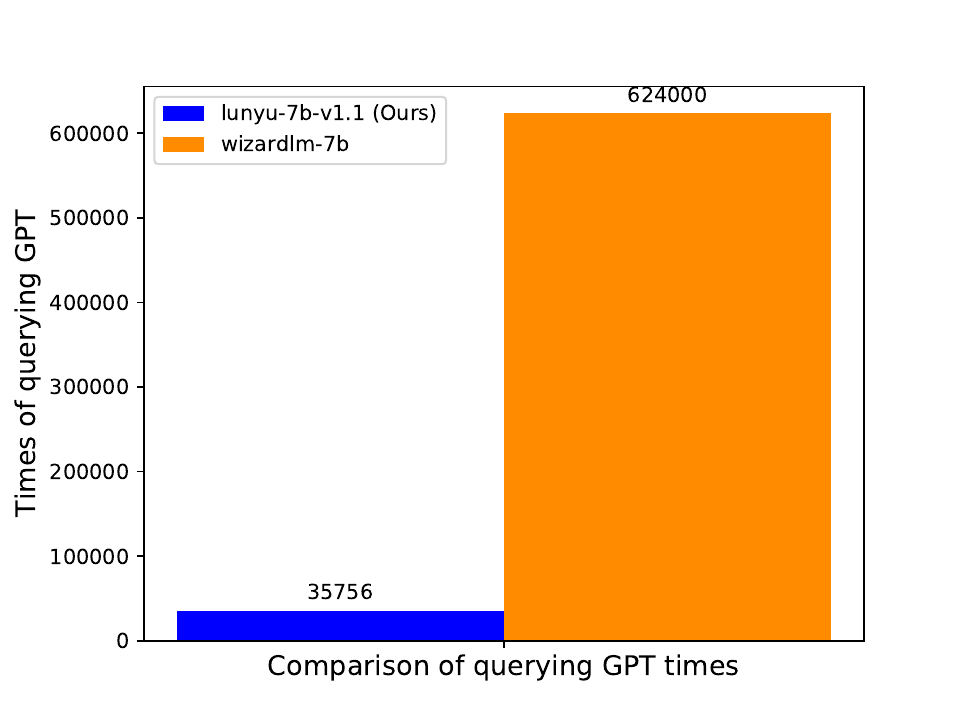}
}
    \vspace{-5pt}
 	\caption{\normalsize Compare with WizardLM 7B on dataset size used for training LLMs and querying times of advanced LLMs. 
 	} 
  \label{fig:compared-with-WizardLM-number-instructions-gpt-ans}
    \vspace{-10pt}
 \end{figure} 
\vspace{-5pt}

\begin{comment}
    \subsection{Experiments of Model Privacy Attack}

\hl{Our objective is to improve model performance while enhancing data privacy, even with limited data. Notably, the TeaMs-RL methodology can effectively mitigate privacy leakage risks typically associated with large datasets. Our experiments clearly demonstrate substantially enhanced privacy protection over the baseline model.} See Appendix~\ref{appendix:model-privacy-attack} for details.
\end{comment}

\begin{comment}
    
\subsection{Generate Instructions with a Trained Policy}

% By leveraging our trained policy, we generate complex instructions with initial instructions and GPT 4 and ChatGPT. The initial instructions are from a popular dataset, Eval dataset\footnote{\url{https://github.com/tatsu-lab/alpaca_eval.git}}.

Capitalizing on the policy we have trained, complex instructions are generated by synergizing initial instructions with GPT-4 or GPT-3.5. It is noteworthy that these initial instructions are culled from a well-established and widely-recognized dataset, namely the Alpaca dataset\footnote{\url{https://github.com/tatsu-lab/alpaca_eval.git}}.
For more details, please see Appendix~\ref{appendix:generate-instructions-gpt4} and Appendix~\ref{appenidx:generate-instructions-gpt35}.
\end{comment}

\subsection{Compare with a lama-2-chat-7b model}
\label{sec:lama2}
\begin{figure}[tb!]
 \centering
 % \vspace{-30pt}
 % \subcaptionbox{}
 {
\includegraphics[width=0.99\linewidth]{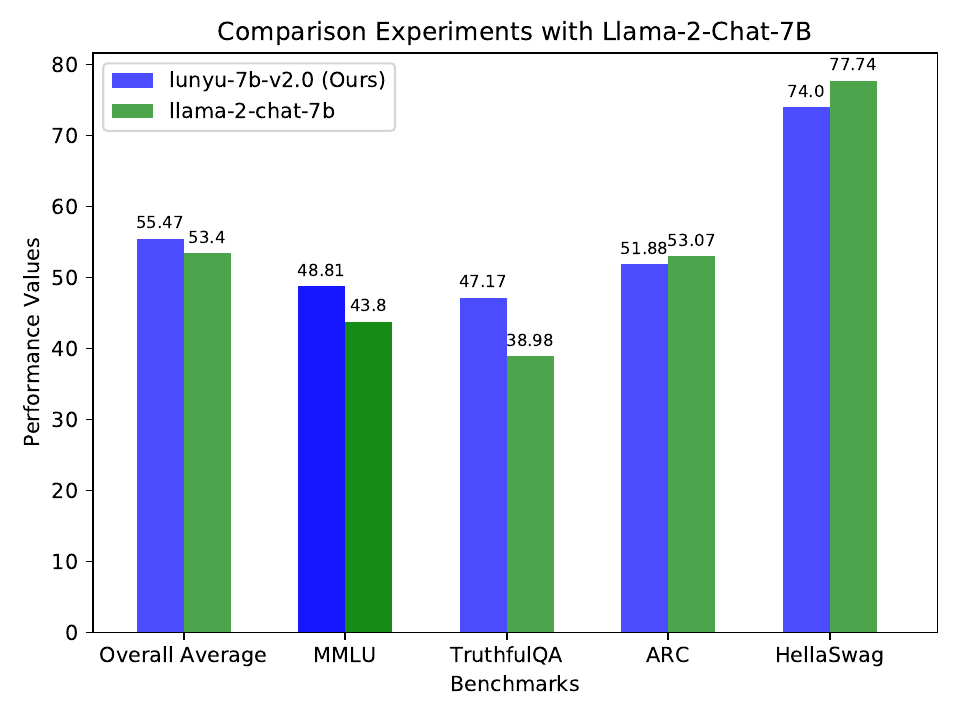}
}
%  {
% \includegraphics[width=0.47\linewidth]{files/figures/compare-WizardLM-llama/compare_TeaMs-RL_WizardLM_llama1.pdf}
% }
    \vspace{-10pt}
 	\caption{\normalsize Compare our method with llama-2-chat-7b on LM-Eval Benchmarks.  
 	} 
  \label{fig:compared-with-llama-2-chat-7b}
  \vspace{-10pt}
 \end{figure} 
 % \vspace{-40pt}
 
We conducted a comparative analysis in the evaluation involving our methodology and Llama-2-chat-7b\footnote{\url{https://huggingface.co/meta-llama/Llama-2-7b-chat-hf}}. As illustrated in Figure \ref{fig:compared-with-llama-2-chat-7b}, we trained a model, denoted as ``TeaMs-RL-7b-v2.0," based on the llama-2-chat-7b architecture using our dataset, encompassing a total of 15,392 instructions along with their corresponding responses. The results of our experimental evaluation reveal noteworthy insights: our model outperforms the llama-2-chat-7b model across several performance metrics, demonstrating superior overall performance. Notably, our methodology exhibits a particularly substantial advantage in tasks related to MMLU and TruthQA, where it exhibits a significant performance edge over the llama-2-chat-7b model.
